# Supplementary material for: Attentive Graph-based Text-aware Preference Modeling for Top-N Recommendation
Source: arXiv:2305.12976 source file (2023-05-22)
Supplement: Supplementary file 1 [file 6_appendix.tex]

\section{Appendix}
\subsection{Reproducibility}\label{sec:reprod}
We list the hyper-parameter settings of training the Autoencoder in \textit{textual content modeling} in Table~\ref{tab:appendix-1}. The hyper-parameters include learning rate $\rho_1$, $L_2$ regularization coefficient $\lambda_1$, batch size $b_1$, number of epochs $n_1$, and hidden size of MLP $d_h$.

\begin{table}[H]
\vspace{-5pt}
\caption{Hyper-parameter settings of training the Autoencoder in \textit{textual content modeling}.}\label{tab:appendix-1}
\vspace{-10pt}
\begin{tabular}{ccccc}
\hline
 $\rho_1$ & $\lambda_1$ & $b_1$ & $n_1$ & $d_h$ \\ \hline\hline
$10^{-3}$ &   $10^{-2}$ &   128 &    50 &   384 \\ \hline
\end{tabular}
\vspace{-5px}
\end{table}

We list the hyper-parameter settings of training embeddings in \textit{item-based preference modeling} on the three datasets in Table~\ref{tab:appendix-2}. The hyper-parameters include learning rate $\rho_2$, $L_2$ regularization coefficient $\lambda_2$, batch size $b_2$, and number of epochs $n_2$.

\begin{table}[H]
\vspace{-5pt}
\caption{Hyper-parameter settings of training embeddings in \textit{item-based preference modeling}.}\label{tab:appendix-2}
\vspace{-10pt}
\begin{tabular}{l|cccc}
\hline
                   &          $\rho_2$ &       $\lambda_2$ & $b_2$ & $n_2$ \\ \hline\hline
Amazon-Musics      & $3\times 10^{-3}$ & $1\times 10^{-2}$ & 1024 & 1000 \\ \hline
Amazon-Movies      & $1\times 10^{-3}$ & $1\times 10^{-3}$ & 1024 & 1000 \\ \hline
Amazon-Electronics & $1\times 10^{-3}$ & $1\times 10^{-3}$ & 2048 & 1000 \\ \hline
\end{tabular}
\vspace{-5px}
\end{table}
